# Supplementary material for: Data-Centric and Data-Aware Frameworks for Fundamentally Efficient Data Handling in Modern Computing Systems
Source: arXiv:2109.05881 source file (2021-09-13)
Supplement: Supplementary file 1 [file AppendixB.tex]

% Table~\ref{table_parameters} shows the system parameters we use in our evaluations. 
% \begin{table}[h]
%   \caption{System configuration.}
%   \vspace{-8pt}
%   \centering
%   \footnotesize
%   \tempcommand{1.3}
%   \renewcommand{\arraystretch}{0.8}
%   \resizebox{\columnwidth}{!}{
%   \begin{tabular}{@{} l @{}}
%   \toprule
%   \textbf{Intel Skylake CPU}
%   x86, 16-cores, 8-wide, out-of-order, 4 GHz  \\
%   L1 Data + Inst. Cache: 32~KB, 8-way 64~B line, LRU policy; \\
%   L2 Cache: Private, 256~KB, 8-way, 64~B line, LRU policy; \\
%   L3 Cache Shared 8 MB (16-banks), 2.5 MB per bank, 16-way\\
%   \midrule
%   \textbf{NVidia Titan V GPU} 6 Graphic Processing Clusters,  80 Streaming Multiprocessors; \\ 
%   5120 Cuda Cores, 1.2 GHz Base Clock, 4.5 MB L2 Cache, 12 GB HBM \\
%   \midrule
%   \textbf{Memory Controller}  8 KB row size, FR-FCFS~\cite{mutlu2007stall} scheduling \\
%   \midrule
%   \textbf{Main memory} DDR4-2400, 1-channel, 1-rank, 16 banks; \\
%   \bottomrule
%   \end{tabular}
%   }
%   %% TRY caption here?
%   \label{table_parameters}
% \end{table}




% \noindent

% \textbf{Description of Evaluated Real-World Applications.}
% \newline


% \noindent{ \textbf{Convolution Neural Networks (CNNs).} \geraldo{CNNs are used in many classification tasks (not only) including image and handwriting classification. \nastaran{CNNs are often} computational \nastaran{intensive} as they use many general-matrix-multiplication (GEMM) operations over float-point operations for each convolution. 
% Prior works~\cite{rastegari2016xnor, lin2017towards, he2020sparse} demonstrate that %they can reduce the high cost of execution convolutions by quantizing both weights and inputs of the network. These networks are called Binary-Weight Network (BWN)~\cite{lin2017towards} and XNOR-Net~\cite{rastegari2016xnor}. Thus, to compute a multiplication-less convolution, these works use
% \nastaran{ using a series of binary bitcount, addition, shift, and XNOR operations, convolutions can be performed without costly multiplications}. In this work, we use the XNOR-NET~\cite{rastegari2016xnor} implementations of VGG-13, VGG-16, and LeNET provided by \cite{he2020sparse}.  We modify their implementation to make use of SIMDRAM bitcout, addition, shift, and XNOR operations. Then, we evaluate the three networks \revBMicro{for inference} using two different datasets: VGG-13 and VGG-16 (using CIFAR-10~\cite{krizhevsky2010convolutional}), and LeNet-5 (using MNIST~\cite{deng2012mnist}).}}

% \geraldo{\noindent{\textbf{k-Nearest Neighbors Classifier (kNN).} An alternative to the Handwritten Digits Recognition problem is to employ a classifier rather than a CNN. Different from CNNs, the kNN does not require long training epochs since it does not need to learn any information from the data. Instead, it simply finds a group of k objects in the training set using simple distance algorithms, as Euclidean distance. We use SIMDRAM to implement the Euclidean distance algorithm in DRAM. We evaluate a kNN algorithm using the MNIST dataset with 3000 training images and 1000 testing images.  We quantize the inputs using an 8-bit representation. }}


% \geraldo{\noindent{\textbf{Database.} We evaluate two different database workloads. First, we build on top of Ambit BitWave~\cite{li2013bitweaving} implementation. BitWave exploits fast bitwise operations by storing columns contiguously in memory. Then, we implement a simple table scan query \texttt{‘select count(*) from T where c1 <= val <= c2'} using the BitWave algorithm. Due to Ambit's limitations, it only accelerates the query's predication \texttt{'c1 <= val  c2'} using in-DRAM operations. However, since SIMDRAM can fully leverage majority-based computing, we also accelerate the bitcount operation (\texttt{count(*)}) using in-DRAM operations. Second, we evaluate the performance of the TPC-H~\cite{tpch} scheme using query 01. We follow the column-based data layout employed in \cite{santos2017operand}. This query executes many arithmetic operations, including addition and multiplication. For our evaluation, we use a scale factor of 100. }}

% \geraldo{\noindent{\textbf{Brightness.} We use a simple image brightness algorithm to demonstrate the benefits of SIMDRAM predication operation. The algorithm evaluates if a given brightness value is larger than 0. If so, it takes some actions accordingly. %increases the pixel value of the image by the brightness value. Before assigning the new brightness value to the pixel, the algorithm verifies if the new pixel value is between 0 and 255.  
% In our SIMDRAM implementation, we use both addition and predication operations. }}




% \newline
% \noindent
% \textbf{Operand-to-Row Mapping Algorithm}


% \ignore{
% \begin{algorithm}[h]
%   %\caption{Find an mapping for a given \texttt{MIG}}
%   \caption{\juang{\mech's Operand-to-Row Mapping.}}
%      \label{alg_mapping}

%   \begin{algorithmic}[1]


%     \State Input: MIG \texttt{G} = (\texttt{V}, \texttt{E})
%     \State $commonRegisters \gets \{T0, T1, T2, T3\} $
%     \State $dualContactRegisters \gets  \{DCC0, DCC1\} $
    
%     \State $allocationMap \gets \emptyset$
%     \State $phase  = 0$
%      \vspace{1em}
  
%     \ForEach{level in \texttt{G}}
%         \ForEach{\texttt{V} in \texttt{G}[level]}
%           \State $negativeOutput = E.output.isNegative$
          
%           \ForEach{input in \texttt{E}}
            
%                 \If{input.is\_negative == $True$}
%                     \State $ava\_reg= dualContactRegisters.front()$
%                     \State $allocationMap[phase, input, E.output]  \gets ava\_reg$
%                     \State $dualContactRegisters.pop\_front()$
%                     \State $negativeOutput = False$
%                 \Else
%                     \If{$level == 0$}
%                         \State $ava\_reg= commonRegisters.front() $
%                         \State $allocationMap[phase, input, E.output] \gets ava\_reg $
%                         \State $commonRegisters.pop\_front()$   
%                     \Else
%                         \State $has\_parent = False$    
%                         \ForEach{$\texttt{E}.output in allocationMap$}
%                             \If{$\texttt{E}.output == input$} 
%                                     \State $parent = allocationMap[E.output]  $
%                                     \State $allocationMap[phase, input, E.output]  \gets  parent $  
%                                     \State $commonRegisters.remove(parent)$  
%                                     \State $has\_parent = True$ 
%                             \EndIf
%                         \EndFor
                            
%                         \If{$has\_parent == False$}
%                             \State $ava\_reg= commonRegisters.front() $
%                             \State $allocationMap[phase, input, E.output] \gets  ava\_reg $
%                             \State $commonRegisters.pop\_front()$    
%                         \EndIf
%                     \EndIf
%                 \EndIf
%             \EndFor
%         \EndFor
        
      
%         \State $emptyCR = (commonRegisters == \emptyset)$
%         \State $emptyDR = (dualContactRegisters == \emptyset)$
%         \If{emptyCR or emptyDR}
%             \State $phase += 1 $
%             \State $commonRegisters \gets\{T0, T1, T2, T3\}$
%             \State $dualContactRegisters \gets\{DCC0, DCC1\}$
%         \EndIf
%     \EndFor
   
%     \vspace{1em}
%   %\tcc{Simplify data mapping by leveraging banking structure (i.e., reduce the number of RowCopies)}
%     \State $\texttt{simplifyMapping(\&allocationMap, G) }$

%   %\tcc{Generate command sequence}
%   \State $\texttt{generateCommandSequence(\&allocationMap, G) }$

%   \end{algorithmic}
% \end{algorithm}
% }

% \begin{algorithm}[h!]
%   %\caption{Find an mapping for a given \texttt{MIG}}
%   \caption{\juang{\mech's Operand-to-Row Mapping.}}
%      \label{alg_mapping}
% \tiny
% %\footnotesize
% %\scriptsize
%   \begin{algorithmic}[1]

%     \State Input: MIG \texttt{G} = (\texttt{V}, \texttt{E})
%     \State $B\_rows \gets \{T0, T1, T2, T3\} $
%     \State $B\_rows\_DCC \gets  \{DCC0, DCC1\} $
%     \State $input\_output\_map \gets \emptyset$
%     \State $phase  = 0$
%     \vspace{0.5em}
  
%     \ForEach{level in \texttt{G}}
%         \ForEach{\texttt{V} in \texttt{G}[level]}
%             \If{level == 0}
%                 \ForEach{input in \texttt{E[V]}}
%                     \If{input is inverted}
%                         \State Map input to row in $B\_rows\_DCC$
%                     \Else
%                         \State Map input to row in $B\_rows$
%                     \EndIf
%                 \EndFor
%             \Else
%                 \ForEach{input in \texttt{E[V]}}
%                     \State Search for parent 
%                         \If{parent is not in $B\_rows$ or $B\_rows\_DCC$}
%                             \If{parent is inverted}
%                                 \State Map parent to row in $B\_rows\_DCC$
%                             \Else
%                                 \State Map parent to row in $B\_rows$
%                           \EndIf
%                         \EndIf
%                 \EndFor
%             \EndIf
%             %\State Save the set of 3 inputs and row mappings in $input\_output\_map$
%             \State $input\_output\_map[] \gets$ inputs in \texttt{E[V]} and row mappings
%             \If{\texttt{V} is the last vertex in \texttt{G}[level]}
%                 \If{output is inverted}
%                     \State Map output to row in $B\_rows\_DCC$
%                 \Else
%                     \State Map output to row in $B\_rows$
%                 \EndIf
%             \Else
%                 \State Map output to row in $D\_rows$
%             \EndIf
%             \If{$B\_rows$ and $B\_rows\_DCC$ are full}
%                 \State $phase += 1$
%             \EndIf
%         \EndFor
%     \EndFor

%   \end{algorithmic}
% \end{algorithm}


% \juang{The input to Algorithm~\ref{alg_mapping} is a MIG \texttt{G = (V,E)} (line 1), where \texttt{V} is the set of all vertices (i.e., majority gates) in \texttt{G}, and \texttt{E} is the set of inputs and outputs of all \texttt{V} vertices (i.e., \texttt{E[V]} contains the inputs and the output of a vertex \texttt{V}). 
% }
% \juang{The algorithm maintains 1) two data structures ($B\_rows$, $B\_rows\_DCC$) to store information regarding the available compute rows in the B-group (lines 2-3), 2) a data structure ($input\_output\_map$) that stores the operand-to-row mappings for the inputs and output of all vertices (line 4), and 3) a $phase$ variable that keeps track of the current execution phase (line 5). The algorithm proceeds as follows.
% }
% \juang{First, the algorithm iterates in topological order over each vertex \texttt{V} (lines 6-7) to respect data dependencies within the graph.
% }
% \juang{Second, if the vertex \texttt{V} is in level 0 of the graph (line 8), the algorithm maps the inputs to rows in the B-group. If an input is inverted, it is mapped to a DCC row (line 11). If not, it is mapped to one row among T0-T3 (line 13). In runtime, these mappings will be performed with RowClone operations. 
% }
% \juang{Third, if the vertex \texttt{V} is \emph{not} in level 0 of the graph (line 14), the algorithm seeks for the parent of each input (i.e., outputs of vertices in the previous level) (line 16). Parents are already mapped to rows in either the B-group or the D-group. In the second case, the parent needs to be remapped to an available row in the B-group (via RowClone operation in runtime) (lines 17-21).
% }
% \juang{Fourth, the set of 3 inputs and its corresponding mappings to compute rows in the B-group constitute the necessary information to perform a TRA (by issuing an AAP) during runtime. This information is saved in $input\_output\_map$ (line 22). 
% Since the nature of the TRA is destructive (i.e., all input rows end up containing the result of the MAJ operation), the output can be kept in a compute row in the B-group for early reuse (e.g., as an input to a vertex in the next level) or be temporarily saved in an auxiliary row in the D-group (lines 24-30). 
% }
% \juang{Fifth, when all rows in the B-group are busy with inputs of the current level, the execution phase finishes and $phase$ is incremented (line 32). At the end of each phase, the algorithm generates the sequence of AAPs from the information about the sets of 3 inputs and its mappings to compute rows ($input\_output\_map$). In runtime, the sequence of AAPs is issued by the control unit in the memory controller (Section~\ref{sec:mc}). \revdel{They are \emph{micro-operations} of a \emph{micro-program} that implements a \mech operation.} 
% }
